# Supplementary material for: A Survey on Complex Tasks for Goal-Directed Interactive Agents
Source: arXiv:2409.18538 source file (2024-09-27)
Supplement: Supplementary file 1 [file appendix.tex]

\section{}\label{appendix:screenshot}

\begin{figure*}[h]
    \centering
    \includegraphics[width=\linewidth]{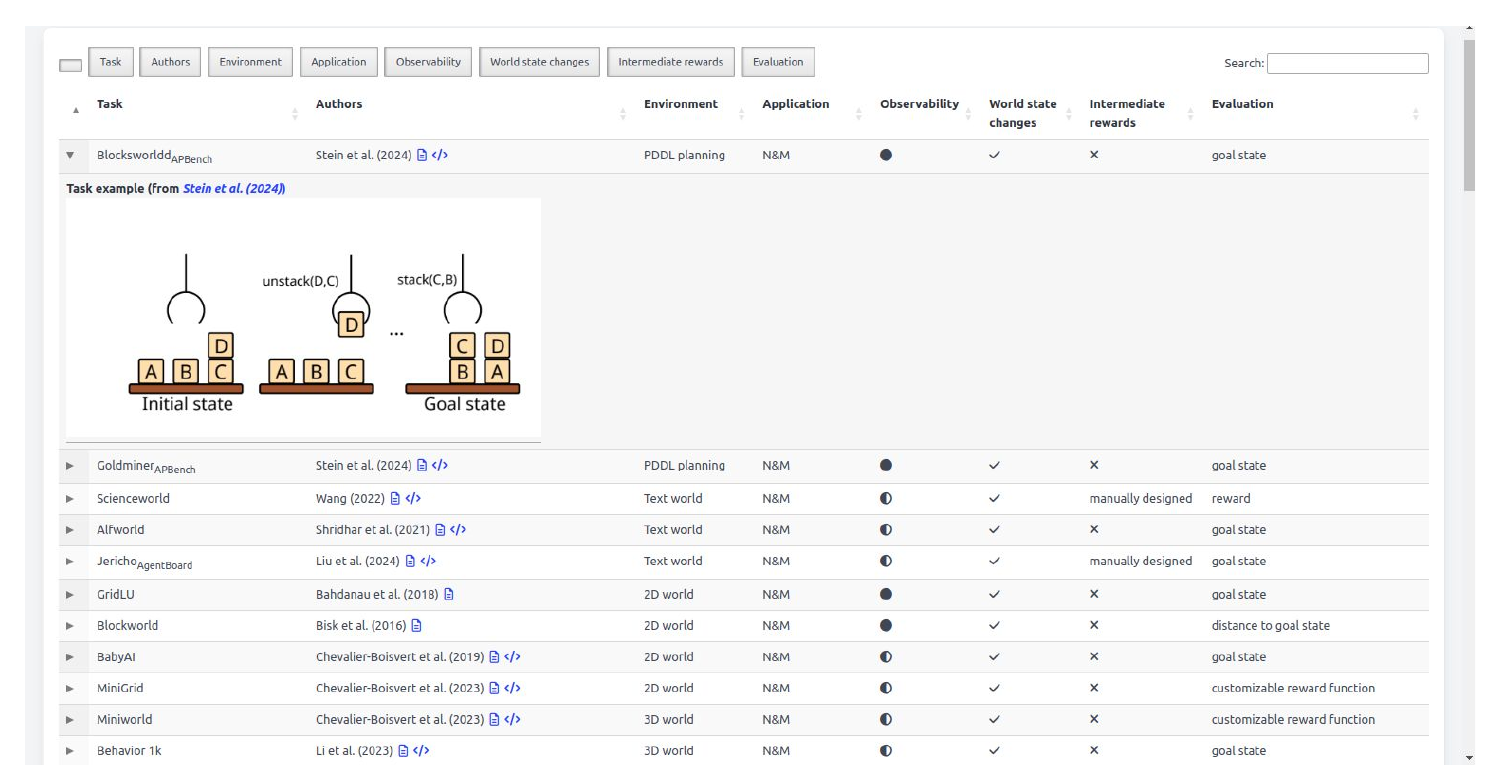}
    \caption{Screenshot of a part of the survey's companion website.}
    \label{fig:screenshot}
\end{figure*}
